# Supplementary material for: Handling Missing Modalities in Multimodal Survival Prediction for Non-Small Cell Lung Cancer
Source: arXiv:2601.10386 source file (2026-04-24)
Supplement: Supplementary file 1 [file TABLES_appendix.tex]

% CT - Tabular
\begin{table*}[h!]
\centering
\caption{
Comparison of \textbf{ConcatODST} and \textbf{CrossAttentionMissingModality} models trained jointly on \textbf{CT–Tabular} modalities (\textbf{Freeze: NO}). 
The table reports mean $\pm$ standard deviation of the concordance index (c-index) across increasing levels of missingness in each modality. 
Each column block corresponds to a prediction target, while rows vary the percentage of missing CT or Tabular inputs. 
}
\scriptsize
\setlength{\tabcolsep}{3.5pt}

\resizebox{\textwidth}{!}{
\begin{tabular}{cc|cc|cc|cc|cc}
\toprule
\
\multirow{2}{*}{\textbf{CT (\%)}} & \multirow{2}{*}{\textbf{Tab (\%)}} &
\multicolumn{2}{c|}{\textbf{OS$_{1d}$}} &
\multicolumn{2}{c|}{\textbf{PFS$_{1d}$}} &
\multicolumn{2}{c|}{\textbf{Local Progression$_{1d}$}} &
\multicolumn{2}{c}{\textbf{M+$_{1d}$}} \\
\cmidrule(lr){3-4} \cmidrule(lr){5-6} \cmidrule(lr){7-8} \cmidrule(lr){9-10}
 & & ConcatODST & CrossAttn & ConcatODST & CrossAttn & ConcatODST & CrossAttn & ConcatODST & CrossAttn \\
\midrule
0 & 0   & 65.24 ± 6.60 & 66.58 ± 4.36 & 52.79 ± 4.29 & 52.71 ± 3.82 & 54.59 ± 8.12 & 58.38 ± 9.76 & 56.95 ± 7.06 & 58.79 ± 6.44 \\
0 & 25  & 59.68 ± 5.32 & 60.72 ± 7.38 & 50.70 ± 4.28 & 49.95 ± 6.27 & 51.13 ± 8.61 & 56.81 ± 14.10 & 50.13 ± 7.96 & 55.96 ± 6.28 \\
0 & 50  & 57.44 ± 3.98 & 55.47 ± 7.85 & 46.24 ± 5.79 & 48.08 ± 6.97 & 54.90 ± 13.48 & 61.32 ± 12.79 & 47.75 ± 8.83 & 54.57 ± 4.97 \\
0 & 75  & 50.50 ± 5.86 & 50.91 ± 4.45 & 49.52 ± 8.61 & 48.19 ± 8.41 & 48.42 ± 12.09 & 61.86 ± 11.33 & 42.50 ± 4.89 & 49.94 ± 7.17 \\
0 & 100 & 50.00 ± 0.00 & 50.00 ± 0.00 & 50.00 ± 0.00 & 50.00 ± 0.00 & 50.00 ± 0.00 & 50.00 ± 0.00 & 50.00 ± 0.00 & 50.00 ± 0.00 \\
25 & 0  & 64.14 ± 6.32 & 64.28 ± 5.97 & 54.35 ± 7.80 & 53.28 ± 5.18 & 52.35 ± 10.62 & 58.04 ± 10.75 & 55.91 ± 6.41 & 63.48 ± 6.54 \\
50 & 0  & 64.11 ± 7.33 & 65.72 ± 5.93 & 51.09 ± 3.99 & 53.58 ± 7.87 & 57.08 ± 9.26  & 57.68 ± 12.76 & 55.10 ± 5.70 & 60.34 ± 6.26 \\
75 & 0  & 63.43 ± 4.74 & 65.31 ± 5.17 & 49.22 ± 6.42 & 53.36 ± 7.98 & 57.99 ± 10.12 & 57.15 ± 11.23 & 57.31 ± 6.85 & 62.83 ± 6.48 \\
100 & 0 & 65.27 ± 5.43 & 66.98 ± 8.00 & 50.01 ± 4.33 & 54.11 ± 5.73 & 53.06 ± 9.97  & 57.69 ± 11.38 & 55.90 ± 5.24 & 62.73 ± 7.46 \\
\bottomrule
\end{tabular}
}
\label{tab:CTTab_nofreeze_results}
\end{table*}

\begin{table*}[h!]
\centering
\caption{
Comparison of \textbf{ConcatODST} and \textbf{CrossAttentionMissingModality} models trained jointly on \textbf{CT–Tabular} modalities (\textbf{Freeze: YES}). 
The table reports mean $\pm$ standard deviation of the concordance index (c-index) for each prediction target across increasing levels of missingness in CT and Tabular inputs. 
Each two-column block corresponds to a target task, allowing assessment of the models' robustness under unimodal information loss.
}

\resizebox{\textwidth}{!}{
\begin{tabular}{cc|cc|cc|cc|cc}
\toprule
\multirow{2}{*}{\textbf{CT (\%)}} & \multirow{2}{*}{\textbf{Tab (\%)}} &
\multicolumn{2}{c|}{\textbf{OS$_{1d}$}} &
\multicolumn{2}{c|}{\textbf{PFS$_{1d}$}} &
\multicolumn{2}{c|}{\textbf{Local Progression$_{1d}$}} &
\multicolumn{2}{c}{\textbf{M+$_{1d}$}} \\
\cmidrule(lr){3-4} \cmidrule(lr){5-6} \cmidrule(lr){7-8} \cmidrule(lr){9-10}
 & & ConcatODST & CrossAttn & ConcatODST & CrossAttn & ConcatODST & CrossAttn & ConcatODST & CrossAttn \\
\midrule
0 & 0   & 65.69 ± 11.13 & 67.75 ± 10.88 & 48.38 ± 7.98 & 49.60 ± 7.11 & 51.76 ± 17.37 & 53.16 ± 16.80 & 55.39 ± 4.68 & 51.67 ± 6.38 \\
0 & 25  & 63.28 ± 12.81 & 67.28 ± 10.16 & 48.62 ± 6.92 & 48.18 ± 6.47 & 51.12 ± 17.21 & 54.30 ± 15.07 & 53.44 ± 4.16 & 47.63 ± 5.56 \\
0 & 50  & 61.17 ± 11.77 & 66.50 ± 10.35 & 47.91 ± 6.43 & 46.40 ± 5.33 & 50.23 ± 14.35 & 55.34 ± 20.38 & 50.26 ± 5.68 & 46.90 ± 4.46 \\
0 & 75  & 60.22 ± 10.75 & 66.92 ± 10.52 & 48.88 ± 8.48 & 45.44 ± 7.07 & 49.63 ± 19.54 & 61.08 ± 13.72 & 49.40 ± 3.74 & 43.94 ± 6.58 \\
0 & 100 & 58.10 ± 12.69 & 64.42 ± 8.56  & 47.93 ± 9.11 & 43.39 ± 7.36 & 51.45 ± 16.66 & 51.38 ± 10.09 & 52.26 ± 8.24 & 45.72 ± 6.57 \\
0 & 0   & 65.69 ± 11.13 & 67.75 ± 10.88 & 48.38 ± 7.98 & 49.60 ± 7.11 & 51.76 ± 17.37 & 53.16 ± 16.80 & 55.39 ± 4.68 & 51.67 ± 6.38 \\
25 & 0  & 65.88 ± 12.40 & 65.49 ± 13.18 & 46.06 ± 6.33 & 50.76 ± 4.61 & 57.63 ± 16.56 & 58.56 ± 14.84 & 56.08 ± 2.09 & 51.16 ± 5.99 \\
50 & 0  & 67.02 ± 10.83 & 67.14 ± 12.87 & 46.99 ± 8.16 & 52.45 ± 5.47 & 57.60 ± 10.60 & 54.66 ± 16.46 & 57.12 ± 4.85 & 51.21 ± 8.74 \\
75 & 0  & 65.91 ± 7.29  & 67.85 ± 7.84  & 47.30 ± 8.80 & 54.14 ± 8.31 & 58.38 ± 13.30 & 58.84 ± 18.11 & 57.14 ± 6.84 & 54.33 ± 4.44 \\
100 & 0 & 66.27 ± 7.54  & 64.24 ± 11.41 & 53.58 ± 6.98 & 57.75 ± 9.64 & 54.33 ± 14.76 & 55.19 ± 13.18 & 58.34 ± 7.10 & 54.74 ± 8.30 \\
\bottomrule
\end{tabular}
}
\label{tab:CTTab_freeze_results}
\end{table*}

% CT - WSI

\begin{table*}[h!]
\centering
\caption{
Comparison of \textbf{ConcatODST} and \textbf{CrossAttentionMissingModality} models trained jointly on \textbf{CT–WSI} modalities (\textbf{Freeze: NO}). 
The table reports mean $\pm$ standard deviation of the concordance index (c-index) across progressive levels of missingness in CT and WSI inputs. 
Each two-column block corresponds to a prediction target, enabling analysis of multimodal robustness when all encoders are trainable.
}

\resizebox{\textwidth}{!}{
\begin{tabular}{cc|cc|cc|cc|cc}
\toprule
\multirow{2}{*}{\textbf{WSI (\%)}} & \multirow{2}{*}{\textbf{CT (\%)}} &
\multicolumn{2}{c|}{\textbf{OS$_{1d}$}} &
\multicolumn{2}{c|}{\textbf{PFS$_{1d}$}} &
\multicolumn{2}{c|}{\textbf{Local Progression$_{1d}$}} &
\multicolumn{2}{c}{\textbf{M+$_{1d}$}} \\
\cmidrule(lr){3-4} \cmidrule(lr){5-6} \cmidrule(lr){7-8} \cmidrule(lr){9-10}
 & & ConcatODST & CrossAttn & ConcatODST & CrossAttn & ConcatODST & CrossAttn & ConcatODST & CrossAttn \\
\midrule
0 & 0   & 61.62 ± 6.43 & 61.45 ± 5.58 & 49.39 ± 10.83 & 55.10 ± 9.49 & 55.45 ± 8.70 & 50.04 ± 10.08 & 55.19 ± 4.99 & 58.05 ± 2.48 \\
0 & 25  & 62.17 ± 7.20 & 62.15 ± 4.37 & 47.31 ± 11.45 & 53.54 ± 7.08 & 53.28 ± 9.96 & 49.51 ± 10.67 & 55.19 ± 6.29 & 58.97 ± 3.74 \\
0 & 50  & 66.21 ± 13.10 & 59.84 ± 8.88 & 49.95 ± 11.65 & 54.38 ± 8.87 & 48.66 ± 9.94 & 45.37 ± 11.19 & 59.29 ± 8.28 & 60.68 ± 6.52 \\
0 & 75  & 61.61 ± 14.16 & 61.65 ± 4.02 & 52.38 ± 11.63 & 56.98 ± 9.01 & 44.84 ± 15.01 & 41.26 ± 15.27 & 60.61 ± 8.77 & 64.67 ± 7.99 \\
0 & 100 & 56.28 ± 12.10 & 53.64 ± 10.23 & 67.47 ± 13.01 & 60.95 ± 16.41 & 51.37 ± 32.84 & 56.78 ± 30.86 & 64.47 ± 9.68 & 74.17 ± 6.30 \\
\midrule[1pt]
0 & 0   & 61.62 ± 6.43 & 61.45 ± 5.58 & 49.39 ± 10.83 & 55.10 ± 9.49 & 55.45 ± 8.70 & 50.04 ± 10.08 & 55.19 ± 4.99 & 58.05 ± 2.48 \\
25 & 0  & 62.06 ± 6.33 & 61.37 ± 5.90 & 48.08 ± 9.46 & 52.26 ± 8.25 & 55.53 ± 8.78 & 50.20 ± 10.00 & 54.92 ± 5.12 & 56.67 ± 1.65 \\
50 & 0  & 62.07 ± 5.51 & 61.64 ± 5.88 & 49.07 ± 10.33 & 53.28 ± 8.49 & 54.66 ± 8.32 & 51.28 ± 10.24 & 57.36 ± 7.00 & 55.97 ± 1.41 \\
75 & 0  & 60.17 ± 6.47 & 56.78 ± 10.82 & 50.92 ± 6.66 & 56.01 ± 6.28 & 55.93 ± 7.15 & 51.73 ± 9.65 & 52.44 ± 4.63 & 53.77 ± 2.77 \\
100 & 0 & 50.00 ± 0.00 & 50.00 ± 0.00 & 50.00 ± 0.00 & 50.00 ± 0.00 & 50.00 ± 0.00 & 50.00 ± 0.00 & 50.00 ± 0.00 & 50.00 ± 0.00 \\
\bottomrule
\end{tabular}
}
\label{tab:CTWSI_nofreeze_results}
\end{table*}

\begin{table*}[h!]
\centering
\caption{
Comparison of \textbf{ConcatODST} and \textbf{CrossAttentionMissingModality} models trained jointly on \textbf{CT–WSI} modalities (\textbf{Freeze: YES}). 
The table reports mean $\pm$ standard deviation of the concordance index (c-index) across increasing levels of missingness in each modality. 
Each two-column block corresponds to a prediction target, while rows vary the percentage of missing CT or WSI inputs, illustrating model robustness under multimodal degradation.
}

\resizebox{\textwidth}{!}{
\begin{tabular}{cc|cc|cc|cc|cc}
\toprule
\multirow{2}{*}{\textbf{WSI (\%)}} & \multirow{2}{*}{\textbf{CT (\%)}} &
\multicolumn{2}{c|}{\textbf{OS$_{1d}$}} &
\multicolumn{2}{c|}{\textbf{PFS$_{1d}$}} &
\multicolumn{2}{c|}{\textbf{Local Progression$_{1d}$}} &
\multicolumn{2}{c}{\textbf{M+$_{1d}$}} \\
\cmidrule(lr){3-4} \cmidrule(lr){5-6} \cmidrule(lr){7-8} \cmidrule(lr){9-10}
 & & ConcatODST & CrossAttn & ConcatODST & CrossAttn & ConcatODST & CrossAttn & ConcatODST & CrossAttn \\
\midrule
0 & 0   & 66.10 ± 5.34 & 64.15 ± 6.77 & 39.81 ± 7.32 & 49.38 ± 7.71 & 58.61 ± 16.14 & 53.99 ± 14.49 & 49.22 ± 10.27 & 44.83 ± 7.62 \\
0 & 25  & 64.99 ± 5.14 & 63.36 ± 3.25 & 41.45 ± 9.44 & 49.77 ± 9.61 & 58.49 ± 21.86 & 53.79 ± 14.91 & 49.86 ± 9.64 & 44.42 ± 8.51 \\
0 & 50  & 62.20 ± 4.23 & 60.64 ± 7.52 & 39.97 ± 11.63 & 53.24 ± 13.65 & 50.60 ± 19.18 & 49.35 ± 14.58 & 58.17 ± 16.28 & 49.70 ± 14.48 \\
0 & 75  & 64.90 ± 10.74 & 57.83 ± 3.64 & 40.48 ± 11.41 & 57.10 ± 11.46 & 54.65 ± 26.86 & 43.34 ± 14.83 & 55.17 ± 12.93 & 45.98 ± 8.67 \\
0 & 100 & 57.89 ± 8.97 & 59.30 ± 15.75 & 47.07 ± 14.32 & 61.61 ± 17.11 & 55.99 ± 29.65 & 62.81 ± 20.69 & 61.92 ± 11.92 & 61.66 ± 16.69 \\
\midrule[1pt]
0 & 0   & 66.10 ± 5.34 & 64.15 ± 6.77 & 39.81 ± 7.32 & 49.38 ± 7.71 & 58.61 ± 16.14 & 53.99 ± 14.49 & 49.22 ± 10.27 & 44.83 ± 7.62 \\
25 & 0  & 65.04 ± 6.14 & 62.30 ± 2.40 & 41.48 ± 8.66 & 51.03 ± 9.72 & 56.10 ± 20.38 & 51.88 ± 14.11 & 48.24 ± 11.16 & 46.42 ± 8.28 \\
50 & 0  & 64.24 ± 4.98 & 64.09 ± 2.95 & 40.66 ± 8.69 & 52.23 ± 9.88 & 53.35 ± 21.14 & 50.54 ± 16.11 & 46.60 ± 6.33 & 47.72 ± 8.28 \\
75 & 0  & 65.23 ± 6.47 & 59.67 ± 4.26 & 43.69 ± 7.24 & 53.25 ± 9.56 & 54.94 ± 21.21 & 55.86 ± 13.47 & 47.67 ± 10.47 & 44.02 ± 9.84 \\
100 & 0 & 64.95 ± 10.32 & 57.20 ± 7.56 & 42.50 ± 4.07 & 50.00 ± 0.00 & 58.90 ± 18.59 & 50.05 ± 11.20 & 43.60 ± 10.91 & 42.03 ± 6.28 \\
\bottomrule
\end{tabular}
}
\label{tab:CTWSI_freeze_results}
\end{table*}

% WSI TABULAR: 
\newpage
\begin{table*}[h]
\centering
\caption{
Comparison of \textbf{ConcatODST} and \textbf{CrossAttentionMissingModality} models trained jointly on \textbf{WSI–Tabular} modalities (\textbf{Freeze: NO}). 
The table reports mean $\pm$ standard deviation of the concordance index (c-index) across four prediction targets under progressive simulated missingness in the WSI and Tabular modalities. 
Each two-column block corresponds to one target task, highlighting the effect of end-to-end fine-tuning on multimodal robustness.
}

\resizebox{\textwidth}{!}{
\begin{tabular}{cc|cc|cc|cc|cc}
\toprule
\multirow{2}{*}{\textbf{WSI (\%)}} &
\multirow{2}{*}{\textbf{Tab (\%)}} &
\multicolumn{2}{c|}{\textbf{OS$_{1d}$}} &
\multicolumn{2}{c|}{\textbf{PFS$_{1d}$}} &
\multicolumn{2}{c|}{\textbf{Local Progression$_{1d}$}} &
\multicolumn{2}{c}{\textbf{M+$_{1d}$}} \\
\cmidrule(lr){3-4}\cmidrule(lr){5-6}\cmidrule(lr){7-8}\cmidrule(lr){9-10}
 &  & ConcatODST & CrossAttn & ConcatODST & CrossAttn & ConcatODST & CrossAttn & ConcatODST & CrossAttn \\
\midrule
0 & 0   & 73.30 ± 7.23 & 72.43 ± 3.41 & 47.38 ± 5.26 & 56.67 ± 6.68 & 52.28 ± 19.91 & 55.00 ± 14.36 & 61.88 ± 5.38 & 66.11 ± 13.12 \\
0 & 25  & 71.80 ± 7.23 & 69.59 ± 7.06 & 52.12 ± 5.14 & 55.59 ± 6.48 & 50.95 ± 21.59 & 51.27 ± 17.78 & 58.46 ± 8.06 & 63.38 ± 11.10 \\
0 & 50  & 69.69 ± 11.16 & 68.20 ± 8.65 & 45.31 ± 4.21 & 52.15 ± 7.58 & 47.80 ± 23.38 & 46.97 ± 22.24 & 58.33 ± 8.29 & 60.83 ± 9.41 \\
0 & 75  & 62.47 ± 10.39 & 61.08 ± 6.69 & 51.28 ± 3.18 & 54.76 ± 6.50 & 45.33 ± 22.67 & 46.86 ± 26.89 & 54.68 ± 3.57 & 58.82 ± 14.10 \\
0 & 100 & 56.61 ± 10.38 & 51.85 ± 13.62 & 57.60 ± 13.88 & 58.76 ± 18.33 & 37.36 ± 26.66 & 57.71 ± 37.69 & 61.98 ± 8.60 & 70.69 ± 8.01 \\
\midrule[1pt]
0 & 0   & 73.30 ± 7.23 & 72.43 ± 3.41 & 47.38 ± 5.26 & 56.67 ± 6.68 & 52.28 ± 19.91 & 55.00 ± 14.36 & 61.88 ± 5.38 & 66.11 ± 13.12 \\
25 & 0  & 71.41 ± 5.40 & 71.30 ± 4.24 & 49.15 ± 9.90 & 55.09 ± 4.98 & 52.64 ± 20.77 & 52.89 ± 18.69 & 62.63 ± 7.16 & 66.15 ± 10.65 \\
50 & 0  & 72.64 ± 6.93 & 70.93 ± 4.33 & 49.17 ± 5.11 & 57.76 ± 5.86 & 51.69 ± 19.94 & 55.33 ± 16.31 & 61.20 ± 8.42 & 64.29 ± 11.15 \\
75 & 0  & 72.72 ± 5.75 & 69.95 ± 3.69 & 48.48 ± 7.95 & 57.21 ± 3.34 & 60.84 ± 15.10 & 56.72 ± 13.74 & 61.29 ± 7.25 & 63.96 ± 9.21 \\
100 & 0 & 67.92 ± 4.90 & 67.21 ± 6.57 & 45.14 ± 7.65 & 49.11 ± 7.00 & 52.90 ± 15.63 & 50.91 ± 13.24 & 59.62 ± 7.33 & 58.78 ± 5.31 \\
\bottomrule
\end{tabular}
}
\label{tab:WSITab_nofreeze_results}
\end{table*}

\begin{table*}[h]
\centering
\caption{
Comparison of \textbf{ConcatODST} and \textbf{CrossAttentionMissingModality} models trained jointly on \textbf{WSI–Tabular} modalities (\textbf{Freeze: YES}). 
The table reports mean $\pm$ standard deviation of the concordance index (c-index) across four prediction targets, under progressive simulated missingness in the WSI and Tabular modalities. 
Each two-column block corresponds to a specific prediction target, illustrating the robustness of frozen multimodal encoders to missing inputs.
}

\resizebox{\textwidth}{!}{
\begin{tabular}{cc|cc|cc|cc|cc}
\toprule
\multirow{2}{*}{\textbf{WSI (\%)}} &
\multirow{2}{*}{\textbf{Tab (\%)}} &
\multicolumn{2}{c|}{\textbf{OS$_{1d}$}} &
\multicolumn{2}{c|}{\textbf{PFS$_{1d}$}} &
\multicolumn{2}{c|}{\textbf{Local Progression$_{1d}$}} &
\multicolumn{2}{c}{\textbf{M+$_{1d}$}} \\
\cmidrule(lr){3-4}\cmidrule(lr){5-6}\cmidrule(lr){7-8}\cmidrule(lr){9-10}
 &  & ConcatODST & CrossAttn & ConcatODST & CrossAttn & ConcatODST & CrossAttn & ConcatODST & CrossAttn \\
\midrule
0 & 0   & 70.63 ± 3.16 & 71.78 ± 8.72 & 48.22 ± 10.08 & 47.38 ± 10.75 & 56.79 ± 13.83 & 54.13 ± 14.57 & 54.16 ± 9.29 & 62.83 ± 5.11 \\
0 & 25  & 67.36 ± 6.09 & 71.47 ± 8.49 & 52.14 ± 10.34 & 51.82 ± 10.49 & 55.42 ± 14.67 & 56.03 ± 12.12 & 52.34 ± 6.29 & 54.63 ± 10.94 \\
0 & 50  & 66.91 ± 9.57 & 68.24 ± 8.43 & 46.05 ± 11.09 & 50.03 ± 16.80 & 56.78 ± 13.51 & 47.73 ± 18.68 & 47.20 ± 9.03 & 55.68 ± 10.42 \\
0 & 75  & 59.63 ± 13.46 & 59.10 ± 13.84 & 51.64 ± 14.99 & 56.32 ± 6.60 & 52.77 ± 19.07 & 43.47 ± 20.28 & 41.24 ± 8.85 & 47.03 ± 13.56 \\
0 & 100 & 53.16 ± 11.46 & 47.13 ± 11.89 & 49.75 ± 21.35 & 54.04 ± 17.09 & 60.09 ± 31.44 & 68.27 ± 23.75 & 46.30 ± 5.57 & 55.12 ± 13.98 \\
\midrule[1pt]
0 & 0   & 70.63 ± 3.16 & 71.78 ± 8.72 & 48.22 ± 10.08 & 47.38 ± 10.75 & 56.79 ± 13.83 & 54.13 ± 14.57 & 54.16 ± 9.29 & 62.83 ± 5.11 \\
25 & 0  & 70.62 ± 6.52 & 70.61 ± 8.76 & 48.66 ± 9.10 & 49.69 ± 10.98 & 60.03 ± 11.53 & 57.43 ± 14.00 & 52.09 ± 8.94 & 61.40 ± 4.43 \\
50 & 0  & 71.41 ± 5.09 & 72.95 ± 10.00 & 46.62 ± 12.72 & 48.59 ± 12.23 & 63.68 ± 12.59 & 53.71 ± 15.39 & 52.77 ± 7.26 & 60.24 ± 8.31 \\
75 & 0  & 70.43 ± 3.78 & 73.81 ± 9.70 & 48.30 ± 8.89 & 48.88 ± 9.94 & 65.98 ± 8.35 & 57.06 ± 15.70 & 52.43 ± 12.16 & 63.11 ± 2.03 \\
100 & 0 & 66.76 ± 7.63 & 65.53 ± 8.96 & 49.57 ± 10.54 & 47.74 ± 7.27 & 67.11 ± 13.54 & 56.96 ± 17.06 & 60.25 ± 4.00 & 60.98 ± 2.97 \\
\bottomrule
\end{tabular}
}
\label{tab:WSITab_freeze_results}
\end{table*}

\newpage
% Trimodal

\begin{table*}[h!]
\centering
\caption{
Comparison of \textbf{ConcatODST} and \textbf{CrossAttentionMissingModality} models trained jointly on \textbf{CT–WSI–Tabular} modalities (\textbf{Freeze: NO}). 
The table reports mean $\pm$ standard deviation of the concordance index (c-index) across four prediction targets under progressive simulated missingness of the WSI, CT, and Tabular modalities. 
Each two-column block corresponds to one target task, illustrating the impact of end-to-end multimodal optimization without frozen encoders.
}

\resizebox{\textwidth}{!}{
\begin{tabular}{ccc|cc|cc|cc|cc}
\toprule
\multirow{2}{*}{\textbf{WSI (\%)}} &
\multirow{2}{*}{\textbf{CT (\%)}} &
\multirow{2}{*}{\textbf{Tab (\%)}} &
\multicolumn{2}{c|}{\textbf{OS$_{1d}$}} &
\multicolumn{2}{c|}{\textbf{PFS$_{1d}$}} &
\multicolumn{2}{c|}{\textbf{Local Progression$_{1d}$}} &
\multicolumn{2}{c}{\textbf{M+$_{1d}$}} \\
\cmidrule(lr){4-5}\cmidrule(lr){6-7}\cmidrule(lr){8-9}\cmidrule(lr){10-11}
 &  &  & ConcatODST & CrossAttn & ConcatODST & CrossAttn & ConcatODST & CrossAttn & ConcatODST & CrossAttn \\
\midrule
0 & 0 & 0   & 70.00 ± 6.67 & 67.40 ± 6.44 & 46.45 ± 7.91 & 46.58 ± 7.34 & 55.05 ± 16.56 & 57.06 ± 16.61 & 59.26 ± 4.97 & 61.19 ± 5.27 \\
0 & 0 & 25  & 67.22 ± 7.82 & 63.96 ± 6.65 & 46.63 ± 12.76 & 47.77 ± 7.55 & 53.92 ± 19.54 & 55.73 ± 17.60 & 53.73 ± 5.40 & 56.91 ± 4.81 \\
0 & 0 & 50  & 63.00 ± 6.07 & 59.55 ± 5.17 & 48.02 ± 12.32 & 47.34 ± 5.14 & 48.22 ± 15.40 & 55.14 ± 19.65 & 47.43 ± 3.21 & 49.16 ± 3.20 \\
0 & 0 & 75  & 62.48 ± 6.12 & 56.25 ± 8.13 & 42.65 ± 7.78 & 42.85 ± 4.06 & 47.19 ± 12.96 & 51.53 ± 12.92 & 43.90 ± 4.51 & 46.54 ± 7.14 \\
0 & 0 & 100 & 59.87 ± 5.59 & 57.44 ± 6.95 & 47.10 ± 10.88 & 44.36 ± 5.71 & 49.83 ± 10.35 & 53.81 ± 8.44 & 50.29 ± 5.16 & 48.50 ± 5.71 \\
\midrule[1pt]
0 & 0 & 0   & 70.00 ± 6.67 & 67.40 ± 6.44 & 46.45 ± 7.91 & 46.58 ± 7.34 & 55.05 ± 16.56 & 57.06 ± 16.61 & 59.26 ± 4.97 & 61.19 ± 5.27 \\
0 & 25 & 0  & 69.91 ± 6.52 & 68.70 ± 8.28 & 43.66 ± 7.01 & 49.84 ± 7.70 & 56.77 ± 15.45 & 53.80 ± 19.49 & 58.95 ± 5.44 & 58.57 ± 3.69 \\
0 & 50 & 0  & 69.36 ± 6.06 & 67.79 ± 4.98 & 46.02 ± 9.60 & 50.12 ± 8.01 & 54.35 ± 14.62 & 58.31 ± 18.38 & 58.52 ± 6.57 & 60.18 ± 3.16 \\
0 & 75 & 0  & 69.30 ± 6.07 & 67.38 ± 5.00 & 43.66 ± 7.00 & 48.49 ± 8.40 & 57.65 ± 14.91 & 56.59 ± 17.81 & 59.06 ± 5.92 & 60.64 ± 3.67 \\
0 & 100 & 0 & 69.96 ± 5.75 & 67.24 ± 5.69 & 44.67 ± 7.19 & 49.94 ± 6.26 & 53.14 ± 15.23 & 58.57 ± 15.91 & 57.49 ± 3.96 & 59.31 ± 4.56 \\
\midrule[1pt]
0 & 0 & 0   & 70.00 ± 6.67 & 67.40 ± 6.44 & 46.45 ± 7.91 & 46.58 ± 7.34 & 55.05 ± 16.56 & 57.06 ± 16.61 & 59.26 ± 4.97 & 61.19 ± 5.27 \\
25 & 0 & 0  & 68.66 ± 6.34 & 67.90 ± 6.82 & 45.01 ± 9.58 & 50.76 ± 5.02 & 53.31 ± 15.37 & 58.72 ± 17.47 & 62.23 ± 7.87 & 58.66 ± 4.51 \\
50 & 0 & 0  & 70.29 ± 6.54 & 65.09 ± 6.87 & 43.19 ± 8.64 & 50.75 ± 7.43 & 55.50 ± 16.56 & 55.73 ± 18.33 & 59.53 ± 5.66 & 61.93 ± 4.73 \\
75 & 0 & 0  & 68.50 ± 5.89 & 67.73 ± 5.84 & 47.11 ± 6.82 & 49.22 ± 5.01 & 58.31 ± 14.54 & 56.81 ± 16.68 & 58.11 ± 6.09 & 58.21 ± 3.55 \\
100 & 0 & 0 & 64.46 ± 7.26 & 61.77 ± 11.30 & 50.57 ± 4.90 & 52.10 ± 11.29 & 55.31 ± 14.23 & 57.82 ± 14.64 & 56.64 ± 9.17 & 62.00 ± 7.81 \\
\bottomrule
\end{tabular}
}
\label{tab:CTWSITab_nofreeze_results}
\end{table*}

\begin{table*}[h!]
\centering
\caption{
Comparison of \textbf{ConcatODST} and \textbf{CrossAttentionMissingModality} models trained jointly on \textbf{CT–WSI–Tabular} modalities (\textbf{Freeze: YES}). 
The table reports mean $\pm$ standard deviation of the concordance index (c-index) for each prediction target, under progressive simulated missingness of the WSI, CT, and Tabular modalities. 
Each two-column block corresponds to one target task, allowing analysis of multimodal robustness when all encoders are frozen.
}

\resizebox{\textwidth}{!}{
\begin{tabular}{ccc|cc|cc|cc|cc}
\toprule
\multirow{2}{*}{\textbf{WSI \n(\%)}} &
\multirow{2}{*}{\textbf{CT (\%)}} &
\multirow{2}{*}{\textbf{Tab (\%)}} &
\multicolumn{2}{c|}{\textbf{OS$_{1d}$}} &
\multicolumn{2}{c|}{\textbf{PFS$_{1d}$}} &
\multicolumn{2}{c|}{\textbf{Local Progression$_{1d}$}} &
\multicolumn{2}{c}{\textbf{M+$_{1d}$}} \\
\cmidrule(lr){4-5}\cmidrule(lr){6-7}\cmidrule(lr){8-9}\cmidrule(lr){10-11}
 &  &  & ConcatODST & CrossAttn & ConcatODST & CrossAttn & ConcatODST & CrossAttn & ConcatODST & CrossAttn \\
\midrule
0 & 0 & 0   & 66.56 ± 9.88 & 71.70 ± 5.20 & 49.32 ± 12.55 & 56.30 ± 12.60 & 51.70 ± 24.40 & 58.36 ± 9.97 & 48.80 ± 11.31 & 55.81 ± 2.93 \\
0 & 0 & 25  & 66.41 ± 8.83 & 72.37 ± 5.99 & 47.49 ± 12.10 & 55.28 ± 14.23 & 52.35 ± 23.25 & 55.34 ± 12.41 & 49.96 ± 11.69 & 54.76 ± 4.74 \\
0 & 0 & 50  & 62.15 ± 10.46 & 68.30 ± 8.93 & 43.58 ± 14.78 & 56.69 ± 10.91 & 46.40 ± 23.24 & 55.58 ± 11.21 & 45.77 ± 5.73 & 51.66 ± 2.96 \\
0 & 0 & 75  & 62.57 ± 10.65 & 65.16 ± 10.77 & 42.60 ± 9.37 & 56.05 ± 8.34 & 47.35 ± 17.14 & 56.08 ± 11.94 & 40.72 ± 7.98 & 54.17 ± 3.64 \\
0 & 0 & 100 & 58.95 ± 9.95 & 68.13 ± 5.79 & 46.37 ± 12.86 & 53.83 ± 9.07 & 46.58 ± 14.27 & 51.32 ± 12.69 & 40.33 ± 10.75 & 56.41 ± 4.95 \\
\midrule[1pt]
0 & 0 & 0   & 66.56 ± 9.88 & 71.70 ± 5.20 & 49.32 ± 12.55 & 56.30 ± 12.60 & 51.70 ± 24.40 & 58.36 ± 9.97 & 48.80 ± 11.31 & 55.81 ± 2.93 \\
0 & 25 & 0  & 67.63 ± 7.73 & 69.42 ± 4.55 & 46.38 ± 13.32 & 57.25 ± 12.00 & 54.48 ± 22.08 & 57.06 ± 11.76 & 53.88 ± 7.75 & 54.78 ± 5.64 \\
0 & 50 & 0  & 69.20 ± 8.13 & 68.15 ± 5.74 & 48.55 ± 12.30 & 56.20 ± 11.35 & 55.30 ± 24.66 & 59.78 ± 13.01 & 59.53 ± 6.21 & 54.95 ± 3.85 \\
0 & 75 & 0  & 69.29 ± 7.66 & 68.13 ± 8.14 & 50.78 ± 9.39 & 55.21 ± 13.47 & 54.80 ± 26.81 & 62.55 ± 15.55 & 53.21 ± 6.37 & 54.15 ± 10.22 \\
0 & 100 & 0 & 69.23 ± 5.75 & 72.90 ± 4.20 & 49.48 ± 10.38 & 58.21 ± 13.07 & 54.82 ± 18.77 & 61.55 ± 11.47 & 63.04 ± 8.53 & 53.79 ± 5.93 \\
\midrule[1pt]
0 & 0 & 0   & 66.56 ± 9.88 & 71.70 ± 5.20 & 49.32 ± 12.55 & 56.30 ± 12.60 & 51.70 ± 24.40 & 58.36 ± 9.97 & 48.80 ± 11.31 & 55.81 ± 2.93 \\
25 & 0 & 0  & 66.78 ± 9.37 & 71.62 ± 5.50 & 43.03 ± 10.21 & 58.13 ± 12.40 & 51.02 ± 19.39 & 52.38 ± 8.28 & 49.52 ± 8.39 & 55.82 ± 4.11 \\
50 & 0 & 0  & 66.15 ± 9.37 & 72.13 ± 6.04 & 44.91 ± 9.18 & 55.75 ± 13.55 & 51.22 ± 22.76 & 57.40 ± 10.55 & 51.61 ± 8.79 & 57.47 ± 4.13 \\
75 & 0 & 0  & 65.87 ± 7.11 & 69.55 ± 7.65 & 47.31 ± 12.41 & 55.77 ± 11.88 & 53.15 ± 20.23 & 56.11 ± 11.07 & 49.56 ± 11.40 & 57.29 ± 7.13 \\
100 & 0 & 0 & 59.46 ± 13.13 & 65.96 ± 5.79 & 49.25 ± 6.46 & 55.78 ± 4.78 & 50.79 ± 13.50 & 52.70 ± 19.13 & 48.86 ± 13.40 & 57.03 ± 3.55 \\
\bottomrule

\end{tabular}
}
\label{tab:CTWSITab_freeze_results}
\end{table*}
